# Supplementary material for: Adversarial Robust Memory-Based Continual Learner
Source: arXiv:2311.17608 source file (2023-11-29)
Supplement: Supplementary file 1 [file appendix.tex]

\usetikzlibrary{mindmap}

%\section{Mind Map}
In the manuscript, we propose the problem of adversarial robust continual learning. Fig.~\ref{fig:mind} shows the overall mind map of the work. Below, we present more details and further discussions.
\begin{figure}
\centering
\begin{tikzpicture}
[
    mindmap,
    concept color = red!30,
    every node/.style = {concept}
]
 
\node {Adversarial Robust Memory-based Continual Learner}
child [grow = 45] {
        node {1. Adversarial Robustness}
            child [grow = 45] {node {\underline{\textbf{Challenge}}: Gradient Obfuscation}
            }
            child [grow = south east] {node {\underline{\textbf{Method}}: Robustness-Aware Experience Reply }
            }
    }
child [grow = south east] {
        node {2. Continual Learning}
            child [grow = 45] {node {\underline{\textbf{Challenge}}: Accelerated Forgetting}
            }
            child [grow =  south east] {node {\underline{\textbf{Method}}: Anti-Forgettable Logit Calibration }
            }
};
\end{tikzpicture}
\caption{The mind map for the proposed adversarial robust memory-based continual learner.}
\label{fig:mind}
\end{figure}

\input{ICCV23_MXY_ARCL/Tables/TinyImageNet}
\section{Training Details}
\subsection{Definations of $p$, $c$, and $u$}
We set $h_{\theta}(x) = [h_{\theta}(x)_{1}, ..., h_{\theta}(x)_{i}, ..., h_{\theta}(x)_{C}]$, where $h_{\theta}(x)_{i}$ means the logit corresponding to the $i$-th class of sample $x$.
If we share classification headers during the total training phase, we can divide the classifier head into three parts: past classes $p$, current classes $c$, and future unseen classes $u$ according to the task order.
\begin{equation}
\begin{aligned}
p =& \{1,2, ..., (t-1)*b\},\\ 
c =& \{(t-1)*b+1, (t-1)*b+2, ... ,t*b\},\\
u =& \{t*b+1,t*b+2,...,C\},
\end{aligned}
\end{equation}
where $b$ is the number of classes of each task.
So we can divide $h_{\theta}(x)$ into three parts: $h_{\theta}(x)_{p}$, $h_{\theta}(x)_{c}$, and $h_{\theta}(x)_{u}$.
$h_{\theta}(x)_{p}$ means the logits of past classes of $x$, $h_{\theta}(x)_{c}$ means the logits of current classes of $x$, and $h_{\theta}(x)_{u}$ means the logits of future classes of $x$.
\subsection{Comparisions with Logit Adjustment} 
Logit adjustment~\cite{menon2021longtail,zhao2022adaptive} is often used in long-tail learning to reduce the negative influence of tail classes from head classes.
Unlike them, we consider future tasks, which are specific to continual learning.

For the negative gradients of the new task data affecting the past tasks, the most related work in continual learning is ER-ACE~\cite{caccia2022new}, which chooses to update the new task with the logit masking to avoid the negative impact on the old task classifier parameters.
ER-ACE can be seen as a special case of our method at the softmax layer, which can be viewed as $\mathrm{v}_{p} = \mathrm{v}_{c} = 0$ for past data, and $\mathrm{v}_{p} = +\infty$, $ \mathrm{v}_{c} = 0$ for current data.
When combined with adversarial training, however, this extreme margin v inhibits the model's ability to learn new knowledge.
% but these methods ignore the fact that the feature extractors are shared, and the old task will still be affected by the gradient of the new task, and the nature of the adversarial sample makes the forgetting of the feature extractors more obvious after adversarial training.
Table~1 also shows that the combination of ER-ACE and AT is worse than ER+AT on adversarial FAA but less forgetting.
% Table2 shows that the combination of our method with AT and TRADES can further improve the robustness of the continual learning model, both in class incremental and task incremental settings. 
% another perspective, ER-ACE can be seen as a special case of our method, which can be viewed as: $v_{pa} = v_{t} = 0$ for past data, and $v_{pa} = +\infty$, $ v_{t} = 0$ for current data.
\input{ICCV23_MXY_ARCL/Figures/RAER}
\subsection{Evaluation Metrics}
%空间有限，这部分准备放Appendix了
To better measure the concerns of both adversarial robustness and continual learning, we computed Final Average Accuracy (FAA) and Forgetting for the adversarial and clean samples, respectively.
Here, we set $a^t_i$ as the accuracy for the $i^{th}$ task after training on task t.
FAA can be defined as:
\begin{equation}
\begin{aligned}
\label{eq:faa}
\mathrm{FAA} \triangleq \frac{1}{T}\sum_{i=1}^T a^T_i,
\end{aligned}
\end{equation}
and forgetting can be defined as:
\begin{equation}
\begin{aligned}
\label{eq:forgetting}
\mathrm{Forgetting} \triangleq \frac{1}{T-1}\sum_{j=1}^{T-1} f_j, \ s.t.\ f_j = \max_{l \in \{1, ..., T-1\}} a^l_i - a^{T}_j.
\end{aligned}
\end{equation}
Forgetting ranges from [-100, 100] and measures the average decrease in accuracy, \textit{i.e.}, the maximum difference in performance with respect to a given task observed over training.
Adversarial samples are generated using both PGD-20 and Auto Attack (AA) attacks for evaluation robustness.

Finally, CRD, FRI, and RRD can be defined as:
\begin{equation}
\begin{aligned}
\label{eq:CRD}
\mathrm{CRD} \triangleq \mathrm{FAA}_{\mathrm{clean}}-\widetilde{\mathrm{FAA}}_{\mathrm{clean}},
\end{aligned}
\end{equation}
\begin{equation}
\begin{aligned}
\label{eq:FRI}
\mathrm{FRI} \triangleq \widetilde{\mathrm{Forgetting}}_{\mathrm{clean}}-\mathrm{Forgetting}_{\mathrm{clean}},
\end{aligned}
\end{equation}
\begin{equation}
\begin{aligned}
\label{eq:RRD}
\mathrm{RRD} \triangleq (\widetilde{\mathrm{FAA}}^{\mathrm{Joint}}_{\mathrm{adv}}-\mathrm{FAA}^{\mathrm{Joint}}_{\mathrm{adv}}) -(\widetilde{\mathrm{FAA}}_{\mathrm{adv}}-\mathrm{FAA}_{\mathrm{adv}}),
\end{aligned}
\end{equation}
where $\mathrm{FAA}_{\mathrm{clean}}$ is clean data FAA of standard continual learner (CL), $\widetilde{\mathrm{FAA}}_{\mathrm{clean}}$ is clean data FAA of adversarial robust continual learner (ARCL); samely $\mathrm{FAA}_{\mathrm{adv}}$ and $\widetilde{\mathrm{FAA}}_{\mathrm{adv}}$ are adversarial data FAA of CL and ARCL, respectively; $\mathrm{Forgetting}_{\mathrm{clean}}$ and $\widetilde{\mathrm{Forgetting}}_{\mathrm{clean}}$ are clean data forgetting of CL and ARCL, respectively $\mathrm{FAA}^{\mathrm{Joint}}$ is the FAA of the joint adversarial learner.
\subsection{Hyper-parameters for Different Baselines}
Both continual learning and adversarial training are hyper-parameter-sensitive domains. To reduce the workload of tuning parameters, we keep the hyper-parameters of the continual learning algorithm consistent with the DER code, and we keep the hyper-parameters of the adversarial training algorithm consistent with their original papers.
\paragraph{ER} For Split-CIFAR10/100 datasets, we set the learning rate as 0.1, batch size as 32, and the number of epochs per task as 50.
\paragraph{DER}For Split-CIFAR10/100 datasets, we set the learning rate as 0.03, batch size as 32, the number of epochs per task as 50, and the $\alpha$ in DER is 0.3.
\paragraph{DER++}For Split-CIFAR10/100 datasets, we set the learning rate as 0.03, batch size as 32, the number of epochs per task as 50, and the $\alpha$ in DER is 0.3. The $\beta$ in DER++ is 0.5 when the buffer size is 200 for Split-CIFAR10 and 500,200 for Split-CIFAR100. When the buffer size is 5120 for Split-CIFAR10, the $\beta$ in DER++ is 1.0.
\paragraph{ER-ACE}For Split-CIFAR10/100 datasets, we set the learning rate as 0.03, batch size as 32, and the number of epochs per task as 50.
\paragraph{Vanilla AT}The learning rate, batch size, and other hyper-parameters associated with the optimization algorithm are all consistent with the combined continual learning algorithm.
When ER+ Vanilla AT combines with ours, the loss of task t can be normalized as:
\begin{equation}
\begin{aligned}
\label{eq:er+at+ours}
L =&\  \mathrm{CE}(\mathrm{softmax}(f^{aflc}_{\theta}({\widetilde{x_t}})),y_{t})\\
&+\mathrm{CE}(\mathrm{softmax}(f^{aflc}_{\theta}({\widetilde{x_{\mathcal{M}}}})),y_{\mathcal{M}}),
\end{aligned}
\end{equation}
and $\alpha$ of AFLC is 1.0 on Split-CIFAR10 dataset, and 8.0 on Split-CIFAR100 dataset.
\paragraph{TRADES}The learning rate, batch size, and other hyper-parameters associated with the optimization algorithm are all consistent with ER algorithm.
When ER+ TRADES combines with ours, the loss of task t can be normalized as:
\begin{equation}
\begin{aligned}
\label{eq:er+trades+ours}
L =&\  \mathrm{CE}(\mathrm{softmax}(f^{aflc}_{\theta}({{x_t}})),y_{t})\\
& + \beta* \mathrm{KL}(f^{aflc}_{\theta}({x_t}),f^{aflc}_{\theta}({\widetilde{x_t})})\\
&+\mathrm{CE}(\mathrm{softmax}(f^{aflc}_{\theta}({{x_{\mathcal{M}}}})),y_{\mathcal{M}})\\
& + \beta* \mathrm{KL}(f^{aflc}_{\theta}({x_\mathcal{M}}),f^{aflc}_{\theta}({\widetilde{x_\mathcal{M}})}),
\end{aligned}
\end{equation}
$\beta$ of TRADES is 6.0, and $\alpha$ of AFLC is 1.0 on Split-CIFAR10 dataset and Split-CIFAR100 dataset.
\paragraph{FAT}The learning rate, batch size, and other hyper-parameters associated with the optimization algorithm are all consistent with ER algorithm.
When ER+ FAT combines with ours, the loss of task t can be normalized as: 
\begin{equation}
\begin{aligned}
\label{eq:er+fat+ours}
L =&\  \mathrm{CE}(\mathrm{softmax}(f_{\theta}({\widetilde{x_t}})),y_{t})\\
&+\mathrm{CE}(\mathrm{softmax}(f_{\theta}({\widetilde{x_{\mathcal{M}}}})),y_{\mathcal{M}}).
\end{aligned}
\end{equation}
Note that when solving the adversarial sample in the training phase, the iteration is stopped once the attack model is successful.
\paragraph{LBGAT}The learning rate, batch size, and other hyper-parameters associated with the optimization algorithm are all consistent with ER algorithm. Here we implement LBGAT based on TRADES ($\beta=0.0$).
When ER+ LBGAT combines with ours, the loss of task t can be normalized as:
\begin{equation}
\begin{aligned}
\label{eq:er+lbgat+ours}
L =&\  \mathrm{CE}(\mathrm{softmax}(f_{\theta}({\widetilde{x_t}})),y_{t})\\
& + \gamma* \mathrm{MSE}(f^{clean}_{\theta}({x_t}),f_{\theta}({\widetilde{x_t})})\\
&+\mathrm{CE}(\mathrm{softmax}(f_{\theta}({\widetilde{x_{\mathcal{M}}}})),y_{\mathcal{M}})\\
& + \gamma* \mathrm{MSE}(f^{clean}_{\theta}({x_\mathcal{M}}),f_{\theta}({\widetilde{x_\mathcal{M}})}),
\end{aligned}
\end{equation}
$\gamma$ of LBGAT is 0.1, and $f^{clean}_{\theta}$ is a standard continual learning model (ER on our experiments) with the model architecture of ResNet-18.

\input{Tables/Ablation2}
\begin{table*}[]
\begin{minipage}{\linewidth}
    \centering
    \centering % 居中显示
    \resizebox{\textwidth}{!}{
    \begin{tabular}{llllllllllll}
    \toprule
    \multirow{3}{*}{\textbf{Buffer Size}} &
    \multirow{3}{*}{\textbf{Methods}} &
    \multicolumn{4}{c}{\textbf{Class Incremental Setting}} &
    \multicolumn{4}{c}{\textbf{Task Incremental Setting}} \\
    ~&~&\multicolumn{2}{c}{\textbf{Clean Data}}&
    \multicolumn{3}{c}{\textbf{Adversarial Data}}&
    \multicolumn{2}{c}{\textbf{Clean Data}}&
    \multicolumn{3}{c}{\textbf{Adversarial Data}}\\
    ~&~&\textbf{FAA$\uparrow$ }&\textbf{Forgetting$\downarrow$}&
    \textbf{PGD-20$\uparrow$}&
    \textbf{AA$\uparrow$}&
    \textbf{Forgetting$\downarrow$}&
    \textbf{FAA$\uparrow$}&
    \textbf{Forgetting$\downarrow$}&
    \textbf{PGD-20$\uparrow$}&
    \textbf{AA$\uparrow$}&
    \textbf{Forgetting$\downarrow$}\\
    \midrule
    {\textbf{200}}&\textbf{ER+Pang~\etal~\cite{pang2022robustness}}& $48.65_{\pm{1.76}}$& $56.79_{\pm{1.78}}$& $2.40_{\pm{0.46}}$& $0.93_{\pm{0.03}}$& $18.96_{\pm{2.47}}$& $88.90_{\pm{2.02}}$& $9.82_{\pm{2.53}}$& $7.25_{\pm{1.06}}$& $6.72_{\pm{0.55}}$& $8.70_{\pm{0.06}}$ \\
    {\textbf{5120}}&\textbf{ER+Pang~\etal~\cite{pang2022robustness}}& $51.37_{\pm{6.44}}$& $52.84_{\pm{8.47}}$& $3.14_{\pm{0.49}}$&$1.10_{\pm{0.05}}$& $20.29_{\pm{2.92}}$& $95.63_{\pm{0.17}}$& $1.58_{\pm{0.21}}$& $14.66_{\pm{0.15}}$&$13.92_{\pm{0.04}}$& $2.53_{\pm{0.46}}$\\
\bottomrule
\end{tabular}}
\subcaption{Results on Split-CIFAR10. We chose two buffer sizes of $200$ and $5120$.}
    \label{Pang-CIFAR10}
\end{minipage}

\begin{minipage}{\linewidth}
    \centering % 居中显示
    \resizebox{\textwidth}{!}{
    \begin{tabular}{llllllllllll}
    \toprule
    \multirow{3}{*}{\textbf{Buffer Size}} &
    \multirow{3}{*}{\textbf{Methods}} &
    \multicolumn{4}{c}{\textbf{Class Incremental Setting}} &
    \multicolumn{4}{c}{\textbf{Task Incremental Setting}} \\
    ~&~&\multicolumn{2}{c}{\textbf{Clean Data}}&
    \multicolumn{3}{c}{\textbf{Adversarial Data}}&
    \multicolumn{2}{c}{\textbf{Clean Data}}&
    \multicolumn{3}{c}{\textbf{Adversarial Data}}\\
    ~&~&\textbf{FAA$\uparrow$ }&\textbf{Forgetting$\downarrow$}&
    \textbf{PGD-20$\uparrow$}&
    \textbf{AA$\uparrow$}&
    \textbf{Forgetting$\downarrow$}&
    \textbf{FAA$\uparrow$}&
    \textbf{Forgetting$\downarrow$}&
    \textbf{PGD-20$\uparrow$}&
    \textbf{AA$\uparrow$}&
    \textbf{Forgetting$\downarrow$}\\
    \midrule
    {\textbf{500}}&\textbf{ER+Pang~\etal~\cite{pang2022robustness}}& $16.22_{\pm{0.63}}$& $77.71_{\pm{0.44}}$& $0.91_{\pm{0.05}}$& $0.62_{\pm{0.00}}$& $6.13_{\pm{0.16}}$& $68.87_{\pm{0.25}}$& $11.21_{\pm{0.73}}$& $3.23_{\pm{0.42}}$& $7.95_{\pm{0.06}}$& $4.94_{\pm{0.05}}$\\
{\textbf{2000}}&\textbf{ER+Pang~\etal~\cite{pang2022robustness}}& $30.10_{\pm{0.53}}$& $61.51_{\pm{1.00}}$& $0.75_{\pm{0.22}}$&$0.51_{\pm{0.02}}$& $4.10_{\pm{0.60}}$& $76.90_{\pm{0.44}}$& $19.60_{\pm{0.32}}$& $4.88_{\pm{0.24}}$&$11.97_{\pm{0.26}}$& $5.25_{\pm{0.20}}$\\
    \bottomrule
    \end{tabular}}
    \subcaption{Results on Split-CIFAR100. We choose two buffer sizes of $500$ and $2000$.}
    \label{Pang-CIFAR100}
\end{minipage}

 \caption{Experiment results on Split-CIFAR10/100 dataset and model architecture is ResNet18.
    Here PGD-20 and are adversarial data Final Average Accuracy (FAA) generated by PGD-20. Forgetting of adversarial data is computed based on PGD-20.}
\label{PangCIFAR}
\end{table*}

\input{Figures/Gradient_norm}
\begin{table}[h]
    \resizebox{0.48\textwidth}{!}{
    \begin{tabular}{lllll}
    \toprule
    \textbf{Method}&
    \textbf{S-CIFAR10~200}&
    \textbf{S-CIFAR10~5120}&
    \textbf{S-CIFAR100~500}&
    \textbf{S-CIFAR100~2000}\\
    \midrule
    \textbf{ER+TRADES}& $7.55$ &$17.90$&$3.73$&$4.41$ \\
    \textbf{ER+TRADES+Ours} & \pmb{$17.49$}&\pmb{$26.11$}&\pmb{$9.61$}&\pmb{$11.06$} \\
\bottomrule
\end{tabular}}
\caption{Defense success rate under black-box attack RayS.
   % The table header is (Dataset~Buffer size).
    % and the number in the table is final average RayS defense accuracy. Limited by computing resources, algorithms run only once. Others are the same as our paper.
    }
    \label{RayS}
\end{table}
\subsection{Adaptive Attack}
For both PGD-20 and AA, we considered both class incremental setting and task incremental setting, and the logit in solving the adversarial sample is processed by AFLC, which we have included in the code section ($adversarial\_attack.py$ and file directory $autoattack\_adaptive$) in the supplementary materials.
\begin{equation}
\begin{aligned}
\label{eq:logit-adjust}
h^{\mathrm{aflc}}_{\theta}(\widetilde{x})_{i} = h_{\theta}(\widetilde{x})_{i} - \alpha \mathrm{v}_i,
\end{aligned}
\end{equation}
where $\mathrm{v}_i$ is the same as the $\mathrm{v}$ of the last task training phase.
\section{More Details of RAER}
\paragraph{Schematic Diagram}

As shown in Figure~\ref{fig:raer}, RAER is effective because 1. Samples that are adversarially safe are selected and the model is more likely to remember them; 2. Data with too large k values are excluded, they are usually close to or even beyond the task boundary to which they belong, and selection among the remaining data can better depict the data distribution and alleviate gradient obfuscation.
\paragraph{Ablation Experiments about $\rho$}
We ablate $\rho$ on the basis of ER+TRADES with a dataset of Split-CIFAR10 and a buffer size of 200. The results are shown in Table~\ref{Ablation2}.
The value of $\rho$ in the range of $[5,10]$ is robust and ensures the selection of safe and diverse samples for storage, but when the parameter $\rho$ is too small $(1)$, the samples selected are safe but not diverse enough to improve the robustness of the model to a limited extent.
We can also find that adding only RAER does not help the robustness of the class incremental setting, because the adversarial sample is too suppressed for the past category, and the robustness in class incremental is improved when AFLC is added (as shown in Table 3 in the paper).

% Due to the tight timeline, the results of $\{\rho = 10, 5, 1\}$ experiments are run two times on different random seeds, and the mean and
% standard deviation are calculated. For a fair comparison, for the experimental results for $\rho=11$ we also only show the variance and the mean of the two times results for the same set of random seeds, so it is not consistent with the results in Table 3 (the results in Table 3 were run three times).
% We have also tried selecting only hard samples, \textit{i.e.}, selecting $k \geq 5$ samples to store, with significantly worse results, which we suspect is because storing only hard samples promotes overfitting.

\section{Differences between Adversarial and Clean Samples}
\paragraph{Gradient Norm}We perform statistics on the gradient norm brought to the classification head by the training process of ER+Vanilla AT for the adversarial and clean samples in the dataset Split-CIFAR10, with a buffer size of 200.
As shown in Fig.~\ref{fig:gn}, both current task data and memory data show that adversarial data bring greater gradients than clean data.

% \paragraph{Logits of Different Classes}明天如果还有空再弄吧

\section{Experimental Results}
\paragraph{New Baseline}
Here we provide a new adversarial training baseline~\cite{pang2022robustness} results. As shown in Table~\ref{PangCIFAR}. Compared with ER+TRADES, it performs better on clean samples but is less adversarial robust, probably because the hyper-parameters are not suitable for continual learning scenarios. We implement it based on ER + TRADES ($\beta = 4.0$), label smoothing is 0.1, and gradient clip is 0.

\paragraph{New Dataset}
Due to the tight timeline, we only choose ER+TRADES as the baseline. Table~\ref{Main-TinyImg} demonstrates the effectiveness of our method in the case of FAA of adversarial/clean samples and anti-forgetting on the Split-Tiny-ImageNet~\cite{stanford2015tinyimagenet} dataset. The results of all experiments are run two times on different random seeds, and the mean and standard deviation are calculated.

Split-Tiny-ImageNet has $200$ classes, each with a training set of 500 samples per class, a validation set of 500 samples per class, and a test set of 500 samples per class. In the continual learning setting, Split-Tiny-ImageNet is divided into $10$ tasks, each of which is a separate $20$ classification task. Following~\cite{buzzega2020dark}, the training epoch per task is $100$, others are the same as Split-CIFAR100.

\paragraph{More Black-box Attack Method}
AA used in our experiments contains a query-efficient black-box attack, Square~\cite{ACFH2020square}.
What's more, we additionally test the robustness of our model against another strong black-box attack, RayS~\cite{chen2020rays} (query limitation is $10,000$).
As shown in Table~\ref{RayS}, our method can effectively improve the robustness of the continual learners under black-box attacks. 
%We only show class-il results due to computational limitations.

% \paragraph{Average Accuracy}
% \input{ICCV23_MXY_ARCL/Tables/Acc_per_task}
% \subsection{Final Accuracy}
% \subsection{Average Accuracy of Different Training Stages}明天再弄
% \subsection{Forward Transfer}
% \subsection{Backward Transfer}
