# Supplementary material for: Adversarial Robust Memory-Based Continual Learner
Source: arXiv:2311.17608 source file (2023-11-29)
Supplement: Supplementary file 2 [file appendix2.tex]

% \clearpage

% \section{Appendix}
\setcounter{equation}{0}
\setcounter{section}{0}
\setcounter{figure}{0}
\setcounter{table}{0}
\usetikzlibrary{mindmap}
% \counterwithout{table}{section}

%\section{Mind Map}
In the manuscript, we propose the problem of adversarial robust continual learning. Fig.~\ref{fig:mind} shows the overall mind map of the work. Below, we present more details and further discussions.
\begin{figure}
\centering
\includegraphics[width=0.5\linewidth]{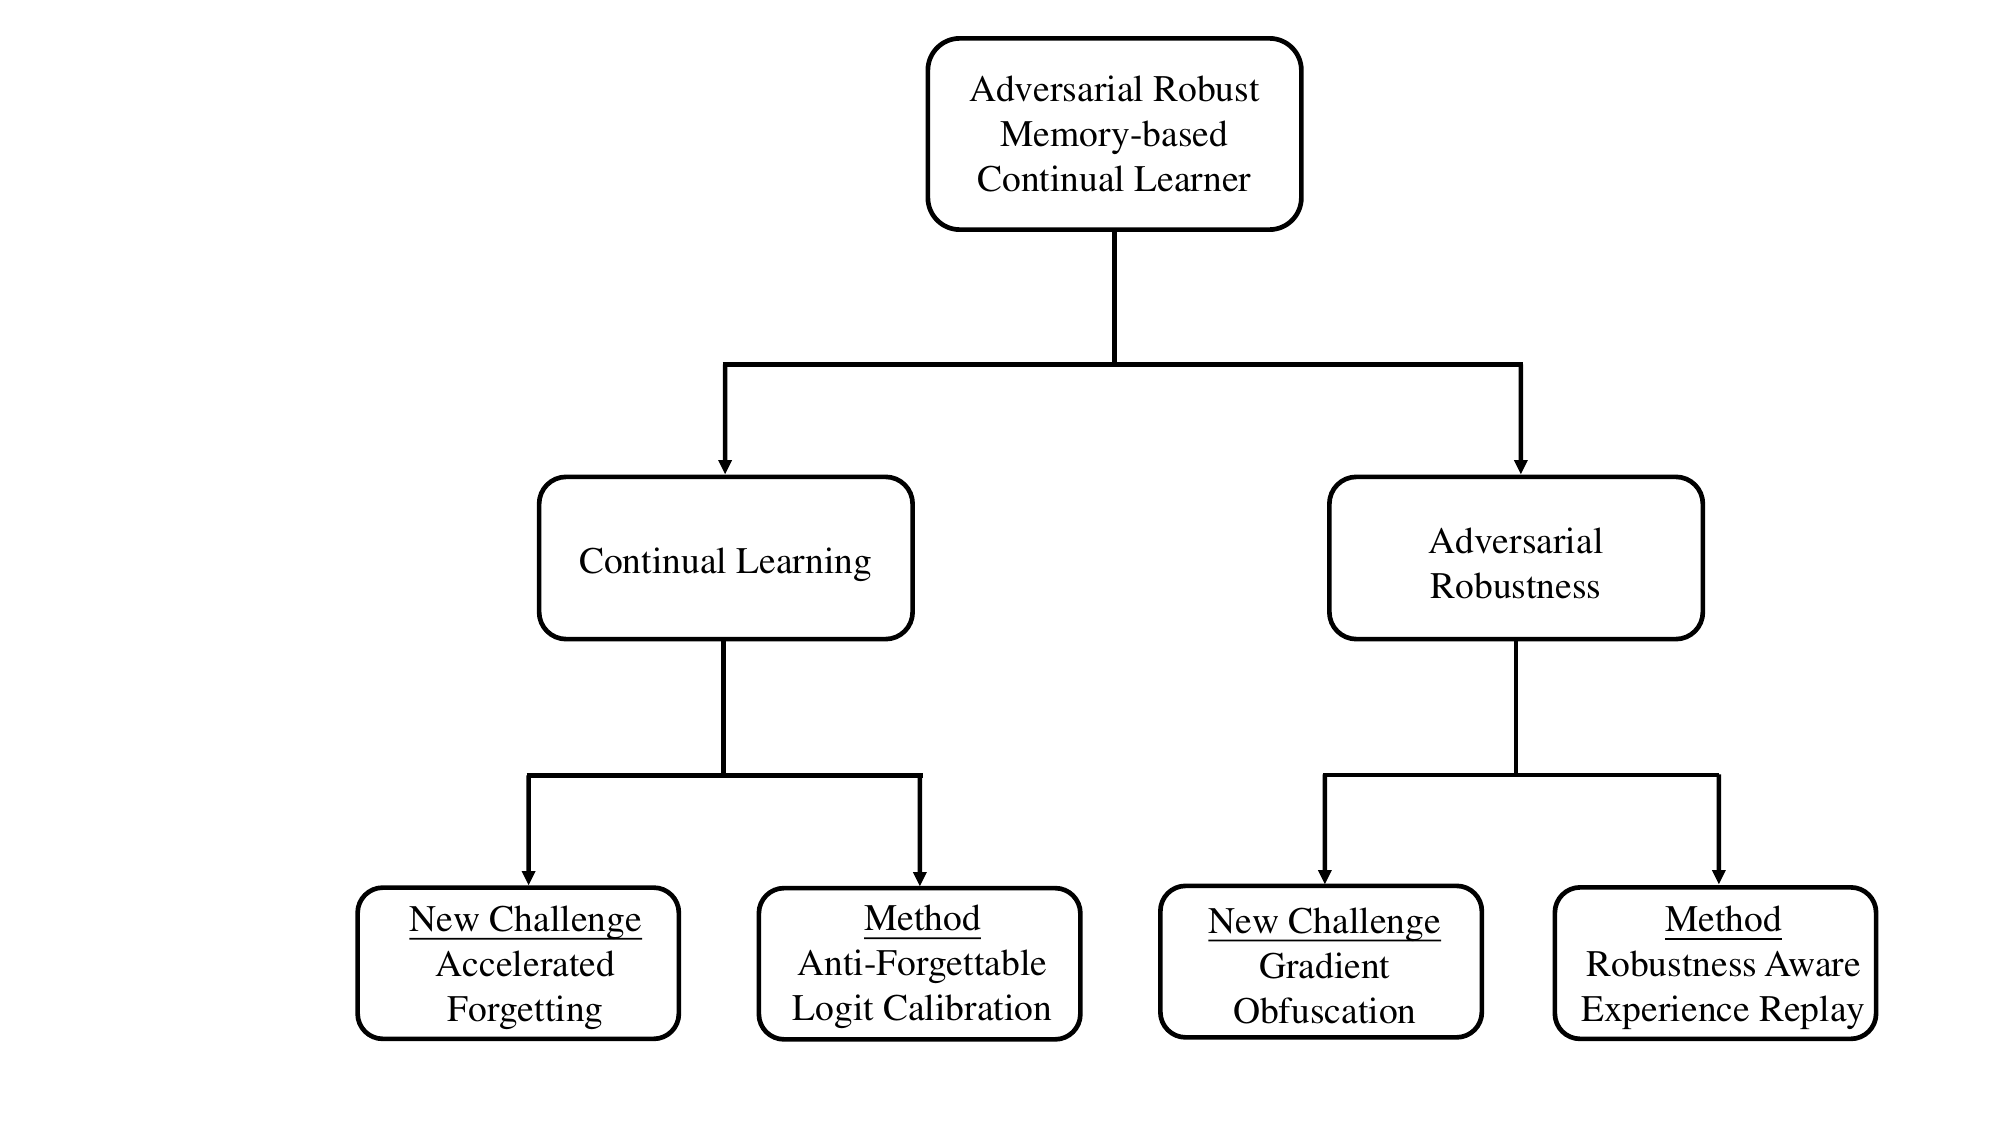}
\caption{The mind map for the proposed adversarial robust memory-based continual learner.}
\label{fig:mind}
\end{figure}
% \begin{figure}
% \centering
% \begin{tikzpicture}
% [
%     mindmap,
%     concept color = red!30,
%     every node/.style = {concept}
% ]
 
% \node {Adversarial Robust Memory-based Continual Learner}
% child [grow = 45] {
%         node {1. Adversarial Robustness}
%             child [grow = 45] {node {\underline{\textbf{Challenge}}: Gradient Obfuscation}
%             }
%             child [grow = south east] {node {\underline{\textbf{Method}}: Robustness-Aware Experience Reply }
%             }
%     }
% child [grow = south east] {
%         node {2. Continual Learning}
%             child [grow = 45] {node {\underline{\textbf{Challenge}}: Accelerated Forgetting}
%             }
%             child [grow =  south east] {node {\underline{\textbf{Method}}: Anti-Forgettable Logit Calibration }
%             }
% };
% \end{tikzpicture}
% \caption{The mind map for the proposed adversarial robust memory-based continual learner.}
% \label{fig:mind}
% \end{figure}

\section{Hyper-parameters in Analysis Experiment}
When the continual algorithms are combined with Vanilla AT (AT), the input of its loss function only changes from clean samples to adversarial samples, so it will not be explained in detail.
\begin{itemize}
    \item \textbf{ER+AT} We set the learning rate as $0.1$, batch size as $32$, and the number of epochs per task as $50$.
    \item \textbf{DER+AT.} We set the learning rate as $0.03$, batch size as $32$, the number of epochs per task as $50$, and the $\alpha$ in DER as $0.3$.
    \item \textbf{DER+++AT.} We set the learning rate as $0.03$, batch size as $32$, the number of epochs per task as $50$, and the $\alpha$ in DER as $0.3$. The $\beta$ in DER++ is $0.5$ when the buffer size is $200$ for Split-CIFAR10 and $500$,$200$ for Split-CIFAR100. When the buffer size is $5120$ for Split-CIFAR10, the $\beta$ in DER++ is $1.0$.
 % \item \textbf{ER-ACE+AT.} We set the learning rate as 0.03, batch size as 32, and the number of epochs per task as 50.
 \item \textbf{X-DER+AT.}  We set the learning rate as $0.03$, batch size as $32$, m as $0.7$, alpha is $0.05$, beta is $0.01$, gamma as $0.85$, lambd as $0.05$, eta as $0.001$, temperature as $5$, batch size of SimCLR loss as $64$, the number of augmentation in SimCLR loss as $2$, and the number of epochs per task as $10$.
\end{itemize}
 
\section{More Experiments}
\noindent \textbf{More Black-box Attack Method.}
AA used in our experiments contains a query-efficient black-box attack, Square~\cite{ACFH2020square}.
What's more, we additionally test the robustness of our model against another strong black-box attack, RayS~\cite{chen2020rays} (query limitation is $10,000$).
As shown in Table~\ref{RayS}, our method can effectively improve the robustness of the continual learners under black-box attacks. 

\begin{table}[h]
\centering
\caption{Defense success rate under black-box attack RayS.
   % The table header is (Dataset~Buffer size).
    % and the number in the table is final average RayS defense accuracy. Limited by computing resources, algorithms run only once. Others are the same as our paper.
    }
    \label{RayS}
    \resizebox{0.48\textwidth}{!}{
    \begin{tabular}{lllll}
    \toprule
    \textbf{Method}&
    \textbf{S-CIFAR10~200}&
    \textbf{S-CIFAR10~5120}&
    \textbf{S-CIFAR100~500}&
    \textbf{S-CIFAR100~2000}\\
    \midrule
    \textbf{ER+TRADES}& $7.55$ &$17.90$&$3.73$&$4.41$ \\
    \textbf{ER+TRADES+Ours} & \pmb{$17.49$}&\pmb{$26.11$}&\pmb{$9.61$}&\pmb{$11.06$} \\
\bottomrule
\end{tabular}}
\end{table}

\begin{table}[]
    
\centering % 居中显示
\caption{Data selection strategy ablation experiments on the CIFAR-10 dataset with the buffer size of 200, using ER + TRADES as the baseline in the class/task incremental settings.
    When $\rho = 11$, this is equivalent to not applying the robust data selection strategy.}
    \label{Ablation2_std}
    \resizebox{0.45\textwidth}{!}{
    \begin{tabular}{lllll}
    \toprule
    \multirow{2}{*}{\textbf{$\rho$}}&
    \multicolumn{2}{c}{\textbf{Class Incremental Setting}}&
    \multicolumn{2}{c}{\textbf{Task Incremental Setting}}\\
    ~&\textbf{FAA$\uparrow$}&
    \textbf{PGD-20$\uparrow$}&
    \textbf{FAA$\uparrow$}&
    \textbf{PGD-20$\uparrow$}\\
    \midrule
    \textbf{$11$}&$22.42_{\pm{7.11}}$& $15.72_{\pm{0.82}}$& $78.79_{\pm{0.81}}$& $51.33_{\pm{2.3}}$\\
    % \textbf{$11$}& $18.32_{\pm{0.47}}$& $83.37_{\pm{2.82}}$& $15.30_{\pm{0.5}}$& $68.17_{\pm{0.08}}$& $78.97_{\pm{1.06}}$& $7.74_{\pm{1.05}}$& $52.64_{\pm{0.67}}$& $21.81_{\pm{1.82}}$\\
    \textbf{$10$}& $18.04_{\pm{0.58}}$& $15.31_{\pm{0.18}}$& $80.38_{\pm{0.16}}$& $59.88_{\pm{1.21}}$ \\
    \textbf{$5$}& $18.21_{\pm{0.25}}$& $15.50_{\pm{0.12}}$& $80.52_{\pm{0.71}}$& $59.50_{\pm{1.82}}$\\
    \textbf{$1$}& $18.35_{\pm{0.88}}$ & $15.06_{\pm{0.17}}$& $79.62_{\pm{0.23}}$& $56.92_{\pm{0.36}}$ \\
    \bottomrule
    \end{tabular}}
    
\end{table}
\begin{table*}[]
    \centering % 居中显示
        \caption{Ablation experiments on the Split-CIFAR10 dataset with the buffer size of $200$, using ER+TRADES as the baseline.  \textbf{Bold} indicates that the inclusion of this module will relatively enhance the corresponding evaluation metrics. Experiments have demonstrated that AFLC mitigates clean-sample accelerated forgetting from adversarial samples, RAER mitigates gradient obfuscation (Adversarial FAA has a boost) and robust forgetting; adding FP improves the model's ability to learn new tasks (FAA has an overall increase).}
    \label{Ablation1_std}
    \resizebox{\textwidth}{!}{
    \begin{tabular}{lllll lll lll}
    \toprule
    \multirow{3}{*}{\textbf{AFLC}} &
    \multirow{3}{*}{\textbf{RAER}}&
    \multirow{3}{*}{\textbf{FP}}&
    \multicolumn{4}{c}{\textbf{Class Incremental Setting}} &
    \multicolumn{4}{c}{\textbf{Task Incremental Setting}} \\
    ~&~&~&\multicolumn{2}{c}{\textbf{Clean Data}}&
    \multicolumn{2}{c}{\textbf{Adversarial Data}}&
    \multicolumn{2}{c}{\textbf{Clean Data}}&
    \multicolumn{2}{c}{\textbf{Adversarial Data}}\\
    ~&~&~&\textbf{FAA$\uparrow$ }&\textbf{Forgetting$\downarrow$}&
    \textbf{FAA$\uparrow$}&
    \textbf{Forgetting$\downarrow$}&
    \textbf{FAA$\uparrow$}&\textbf{Forgetting$\downarrow$}&
    \textbf{FAA$\uparrow$}&\textbf{Forgetting$\downarrow$}\\
    \midrule
    & & &$22.42_{\pm{7.11}}$& $77.25_{\pm{10.79}}$& $15.72_{\pm{0.82}}$& $64.95_{\pm{5.58}}$& $78.79_{\pm{0.81}}$& $8.1_{\pm{0.97}}$& $51.33_{\pm{2.3}}$& $21.97_{\pm{1.31}}$ \\
    % $\usym{2713}$& & & \pmb{$38.85_{\pm{3.26}}$}& \pmb{$47.53_{\pm{21.21}}$}& \pmb{$17.56_{\pm{1.4}}$}& \pmb{$42.80_{\pm{21.82}}$}& \pmb{$82.70_{\pm{0.43}}$}& $9.97_{\pm{1.04}}$& $50.67_{\pm{6.55}}$& $26.28_{\pm{10.45}}$ \\
    $\usym{2713}$ & & & $37.88_{\pm{0.54}}$& $21.76_{\pm{0.23}}$& $18.58_{\pm{1.9}}$& $21.77_{\pm{0.24}}$& $81.66_{\pm{0.02}}$& $10.86_{\pm{0.78}}$& $53.64_{\pm{1.48}}$& $17.6_{\pm{0.28}}$\\
   
    $\usym{2713}$&$\usym{2713}$& &$37.45_{\pm{5.28}}$& \pmb{$10.29_{\pm{11.36}}$}& \pmb{$19.81_{\pm{1.75}}$}& \pmb{$9.61_{\pm{6.38}}$}& $78.13_{\pm{3.1}}$& $15.39_{\pm{4.28}}$& \pmb{$55.71_{\pm{3.47}}$}& \pmb{$14.13_{\pm{3.09}}$} \\
    $\usym{2713}$&$\usym{2713}$&$\usym{2713}$& \pmb{$43.34_{\pm{4.27}}$}& $33.40_{\pm{11.02}}$& \pmb{$19.85_{\pm{1.55}}$}& $30.78_{\pm{8.84}}$& \pmb{$82.59_{\pm{1.12}}$}& \pmb{$7.53_{\pm{1.24}}$}& \pmb{$59.41_{\pm{0.61}}$}& $14.16_{\pm{1.29}}$  \\
\bottomrule
\end{tabular}}

\end{table*}
\begin{table*}[]
    \centering % 居中显示
        \caption{Ablation experiments of different $\alpha$.}
    \label{Ablation3_std}
    \resizebox{\textwidth}{!}{
    \begin{tabular}{l ll lll lll}
    \toprule
    \multirow{3}{*}{\textbf{$\alpha$}}&
    \multicolumn{4}{c}{\textbf{Class Incremental Setting}} &
    \multicolumn{4}{c}{\textbf{Task Incremental Setting}} \\
    ~&\multicolumn{2}{c}{\textbf{Clean Data}}&
    \multicolumn{2}{c}{\textbf{Adversarial Data}}&
    \multicolumn{2}{c}{\textbf{Clean Data}}&
    \multicolumn{2}{c}{\textbf{Adversarial Data}}\\
    ~&\textbf{FAA$\uparrow$ }&\textbf{Forgetting$\downarrow$}&
    \textbf{FAA$\uparrow$}&
    \textbf{Forgetting$\downarrow$}&
    \textbf{FAA$\uparrow$}&\textbf{Forgetting$\downarrow$}&
    \textbf{FAA$\uparrow$}&\textbf{Forgetting$\downarrow$}\\
    \midrule
    
    $0.0$& \pmb{$38.85_{\pm{3.26}}$}& {$47.53_{\pm{21.21}}$}& {$17.56_{\pm{1.40}}$}& {$42.80_{\pm{21.82}}$}& \pmb{$82.70_{\pm{0.43}}$}& \pmb{$9.97_{\pm{1.04}}$} & $50.67_{\pm{6.55}}$& $26.28_{\pm{10.45}}$ \\

    $3.5$& $37.88_{\pm{0.54}}$& $21.76_{\pm{0.23}}$&  \pmb{$18.58_{\pm{1.90}}$}& $21.77_{\pm{0.24}}$& $81.66_{\pm{0.02}}$& $10.86_{\pm{0.78}}$& \pmb{$53.64_{\pm{1.48}}$}& $17.60_{\pm{0.28}}$\\

    $7.0$& $35.92_{\pm{0.88}}$& \pmb{$20.99_{\pm{6.03}}$}& $13.89_{\pm{0.63}}$&  \pmb{$21.76_{\pm{0.67}}$}& $82.56_{\pm{0.58}}$& $10.49_{\pm{3.75}}$& $52.69_{\pm{1.18}}$& \pmb{$16.25_{\pm{2.52}}$}\\

    % $4$& \pmb{$38.85_{\pm{3.26}}$}& \pmb{$47.53_{\pm{21.21}}$}& \pmb{$17.56_{\pm{1.4}}$}& \pmb{$42.80_{\pm{21.82}}$}& \pmb{$82.70_{\pm{0.43}}$}& $9.97_{\pm{1.04}}$& $50.67_{\pm{6.55}}$& $26.28_{\pm{10.45}}$ \\

    % $7$& \pmb{$38.85_{\pm{3.26}}$}& \pmb{$47.53_{\pm{21.21}}$}& \pmb{$17.56_{\pm{1.4}}$}& \pmb{$42.80_{\pm{21.82}}$}& \pmb{$82.70_{\pm{0.43}}$}& $9.97_{\pm{1.04}}$& $50.67_{\pm{6.55}}$& $26.28_{\pm{10.45}}$ \\

    % $10$& \pmb{$38.85_{\pm{3.26}}$}& \pmb{$47.53_{\pm{21.21}}$}& \pmb{$17.56_{\pm{1.4}}$}& \pmb{$42.80_{\pm{21.82}}$}& \pmb{$82.70_{\pm{0.43}}$}& $9.97_{\pm{1.04}}$& $50.67_{\pm{6.55}}$& $26.28_{\pm{10.45}}$ \\
   
\bottomrule
\end{tabular}}

\end{table*}

\begin{table*}[]
    \caption{Experiment results on Split-CIFAR10/100 dataset and model architecture is ResNet18.
    Here PGD-20 and AA are adversarial data Final Average Accuracy (FAA) generated by PGD-20 and Auto Attack (AA) respectively. Forgetting of adversarial data is computed based on PGD-20. With the addition of ours, model performance can be improved across the board.}
    \label{MainCIFAR-var}
\begin{minipage}{\linewidth}
    \centering
    \subcaption{Results on Split-CIFAR10. We chose two buffer sizes of $200$ and $5120$.}
    \label{Main-CIFAR10-var}
    \centering % 居中显示
    \resizebox{\textwidth}{!}{
    \begin{tabular}{llllllllllll}
    \toprule
    \multirow{3}{*}{\textbf{Buffer Size}} &
    \multirow{3}{*}{\textbf{Methods}} &
    \multicolumn{5}{c}{\textbf{Class Incremental Setting}} &
    \multicolumn{5}{c}{\textbf{Task Incremental Setting}} \\
    ~&~&\multicolumn{2}{c}{\textbf{Clean Data}}&
    \multicolumn{3}{c}{\textbf{Adversarial Data}}&
    \multicolumn{2}{c}{\textbf{Clean Data}}&
    \multicolumn{3}{c}{\textbf{Adversarial Data}}\\
    ~&~&\textbf{FAA$\uparrow$ }&\textbf{Forgetting$\downarrow$}&
    \textbf{PGD-20$\uparrow$}&
    \textbf{AA$\uparrow$}&
    \textbf{Forgetting$\downarrow$}&
    \textbf{FAA$\uparrow$}&
    \textbf{Forgetting$\downarrow$}&
    \textbf{PGD-20$\uparrow$}&
    \textbf{AA$\uparrow$}&
    \textbf{Forgetting$\downarrow$}\\
    \midrule
    \multirow{6}{*}{\textbf{200}}&\textbf{ER+AT}& $28.18_{\pm{0.69}}$ & $80.58_{\pm{1.05}}$ & $17.86_{\pm{0.29}}$ &$16.94_{\pm{0.38}}$ & $69.58_{\pm{1.15}}$ & $84.49_{\pm{0.61}}$ & $10.23_{\pm{0.98}}$ & $44.30_{\pm{1.05}}$ & $44.69_{\pm{1.04}}$ & $36.89_{\pm{1.11}}$  \\
    ~&\textbf{ER+TRADES}& $22.42_{\pm{7.11}}$& $77.25_{\pm{10.79}}$& $15.72_{\pm{0.82}}$& $15.53_{\pm{0.68}}$& $64.95_{\pm{5.58}}$& $78.79_{\pm{0.81}}$& $8.10_{\pm{0.97}}$& $51.33_{\pm{2.30}}$& $51.50_{\pm{2.33}}$& $21.97_{\pm{1
.31}}$  \\
    ~&\textbf{ER+FAT}&$33.61_{\pm{6.80}}$ & $69.21_{\pm{8.95}}$ & $15.14_{\pm{0.80}}$ & $14.81_{\pm{0.92}}$ & $49.04_{\pm{7.29}} $& $83.40_{\pm{0.92}}$ & $10.35_{\pm{0.83}}$ & $43.69_{\pm{2.08}}$ & $43.96_{\pm{2.11}}$ & $28.56_{\pm{2.14}}$  \\
 ~&\textbf{ER+LBGAT}& $25.68_{\pm{0.56}}$& $84.47_{\pm{0.63}}$& $16.65_{\pm{0.11}}$& $16.56_{\pm{0.09}}$& $70.5_{\pm{0.29}}$& $78.19_{\pm{1.17}}$& $18.85_{\pm{1.58}}$& $40.69_{\pm{3.03}}$& $40.73_{\pm{3.15}}$& $40.83_{\pm{3.80}}$\\
 ~&\textbf{ER+Pang~\etal~\cite{pang2022robustness}}&  {$48.65_{\pm{1.76}}$} & $56.79_{\pm{1.78}}$& $2.40_{\pm{0.46}}$& $0.93_{\pm{0.03}}$& $18.96_{\pm{2.47}}$& $88.90_{\pm{2.02}}$& $9.82_{\pm{2.53}}$& $7.25_{\pm{1.06}}$& $6.72_{\pm{0.55}}$& $8.70_{\pm{0.06}}$ \\
    \cmidrule(r){2-12}
    ~&\textbf{ER+AT+Ours}& 
    $35.68_{\pm{0.57}}$& $71.18_{\pm{0.66}}$& $18.40_{\pm{0.56}}$& $18.16_{\pm{0.50}}$& $67.85_{\pm{0.72}}$&  {$84.87_{\pm{0.56}}$}& $9.93_{\pm{0.60}}$& $47.30_{\pm{1.31}}$& $47.61_{\pm{1.35}}$& $34.04_{\pm{1.42}}$ \\
    % $47.70_{\pm{0.67}}$&$53.19_{\pm{1.87}}$&$18.20_{\pm{0.02}}$&$17.48_{\pm{0.01}}$&$56.73_{\pm{1.10}}$&$85.40_{\pm{1.28}}$&$9.20_{\pm{1.67}}$&$48.38_{\pm{0.67}}$&$48.54_{\pm{0.75}}$&$31.68_{\pm{1.49}}$\\
    ~&\textbf{ER+TRADES+Ours}& 
    % $42.72_{\pm{0.14}}$&$26.26_{\pm{2.78}}$&$19.73_{\pm{0.64}}$&$17.54_{\pm{0.02}}$&$23.14_{\pm{5.2}}$&$80.64_{\pm{2.45}}$&$9.25_{\pm{1.38}}$&$58.21_{\pm{0.05}}$&$58.53_{\pm{0.01}}$&$15.57_{\pm{0.0}}$\\
     {$43.34_{\pm{4.27}}$} &  {$33.40_{\pm{11.02}}$} &  {$19.85_{\pm{1.55}}$}&   {$18.35_{\pm{1.14}}$} &  {$30.78_{\pm{8.84}}$}& $82.59_{\pm{1.12}}$& { $7.53_{\pm{1.24}}$ }& { $59.41_{\pm{0.61}}$} &   {$59.59_{\pm{0.64}}$ }&  {$14.16_{\pm{1.29}}$}\\
    \cmidrule(r){1-12}
    \multirow{6}{*}{\textbf{5120}}&\textbf{ER+AT} & $61.88_{\pm{0.74}}$ & $37.72_{\pm{0.73}}$ & $27.28_{\pm{0.56}}$ & $26.69_{\pm{0.52}}$ & $41.66_{\pm{1.22}}$ & $91.24_{\pm{0.19}}$ & $2.56_{\pm{0.12}}$ & $56.59_{\pm{0.88}}$ & $56.90_{\pm{0.88}}$ & $19.34_{\pm{1.11}}$\\
    ~&\textbf{ER+TRADES}& $20.36_{\pm{2.81}}$& $85.14_{\pm{4.28}}$& $16.3_{\pm{0.44}}$& $16.18_{\pm{0.35}}$& $72.85_{\pm{1.46}}$& $88.48_{\pm{0.81}}$&  {$1.59_{\pm{0.86}}$} & $64.36_{\pm{0.51}}$& $64.52_{\pm{0.48}}$& $12.47_{\pm{0.37}}$   \\
    ~&\textbf{ER+FAT}& $54.55_{\pm{6.71}}$& $43.18_{\pm{7.51}}$& $19.68_{\pm{2.54}}$& $18.91_{\pm{2.38}}$& $42.15_{\pm{3.59}}$& $91.50_{\pm{0.53}}$& $2.12_{\pm{0.80}}$& $56.72_{\pm{0.65}}$& $56.87_{\pm{0.70}}$& $14.79_{\pm{1.13}}$  \\
    ~&\textbf{ER+LBGAT}& $62.45_{\pm{0.46}}$& $37.73_{\pm{0.97}}$& $27.42_{\pm{0.27}}$& $26.66_{\pm{0.33}}$& $47.83_{\pm{0.49}}$& $91.10_{\pm{0.62}}$& $3.25_{\pm{1.06}}$& $56.57_{\pm{1.02}}$& $56.31_{\pm{1.13}}$& $19.38_{\pm{0.84}}$\\
   ~&\textbf{ER+Pang~\etal~\cite{pang2022robustness}}& $51.37_{\pm{6.44}}$& $52.84_{\pm{8.47}}$& $3.14_{\pm{0.49}}$&$1.10_{\pm{0.05}}$& $20.29_{\pm{2.92}}$& $95.63_{\pm{0.17}}$& $1.58_{\pm{0.21}}$& $14.66_{\pm{0.15}}$&$13.92_{\pm{0.04}}$& $2.53_{\pm{0.46}}$\\
    \cmidrule(r){2-12}
    ~&\textbf{ER+AT+Ours}& 
    $64.34_{\pm{0.68}}$&$23.64_{\pm{0.23}}$&$31.31_{\pm{0.07}}$&$30.49_{\pm{0.06}}$&$20.46_{\pm{0.75}}$&$91.0_{\pm{0.07}}$&$3.51_{\pm{0.14}}$&$60.49_{\pm{0.24}}$&$60.61_{\pm{0.28}}$&$13.27_{\pm{0.33}}$\\
%      {$64.81_{\pm{0.57}}$}&  {$31.73_{\pm{0.86}}$}&  {$29.46_{\pm{0.25}}$}&  {$28.68_{\pm{0.38}}$}&  {$37.62_{\pm{1.37}}$}&  {$91.60_{\pm{0.21}}$}& $2.37_{\pm{0.20}}$& $60.04_{\pm{0.83}}$& $60.34_{\pm{0.87}}$& $16.26_{\pm{0.
% 56}}$ \\
   ~&\textbf{ER+TRADES+Ours} & 
% $42.12_{\pm{0.88}}$&$1.57_{\pm{1.67}}$&$28.37_{\pm{0.09}}$&$30.33_{\pm{1.78}}$&$1.48_{\pm{0.43}}$&$85.55_{\pm{0.01}}$&$7.02_{\pm{0.04}}$&$67.88_{\pm{0.03}}$&$67.97_{\pm{0.04}}$&$3.81_{\pm{2.33}}$\\
   $39.80_{\pm{12.23}}$& $44.08_{\pm{18.66}}$& $23.07_{\pm{6.10}}$& $21.98_{\pm{5.41}}$& $41.37_{\pm{11.41}}$& $86.48_{\pm{2.55}}$& $1.71_{\pm{0.62}}$&  {$69.25_{\pm{2.23}}$} &  {$69.38_{\pm{2.23}}$} & {$5.33_{\pm{0.74}}$}\\
\bottomrule
\end{tabular}}
\end{minipage}
 
\begin{minipage}{\linewidth}
    \subcaption{Results on Split-CIFAR100. We choose two buffer sizes of $500$ and $2000$.}
    \label{Main-CIFAR100-var}
    \centering % 居中显示
    \resizebox{\textwidth}{!}{
    \begin{tabular}{llllllllllll}
    \toprule
    \multirow{3}{*}{\textbf{Buffer Size}} &
    \multirow{3}{*}{\textbf{Methods}} &
    \multicolumn{5}{c}{\textbf{Class Incremental Setting}} &
    \multicolumn{5}{c}{\textbf{Task Incremental Setting}} \\
    ~&~&\multicolumn{2}{c}{\textbf{Clean Data}}&
    \multicolumn{3}{c}{\textbf{Adversarial Data}}&
    \multicolumn{2}{c}{\textbf{Clean Data}}&
    \multicolumn{3}{c}{\textbf{Adversarial Data}}\\
    ~&~&\textbf{FAA$\uparrow$ }&\textbf{Forgetting$\downarrow$}&
    \textbf{PGD-20$\uparrow$}&
    \textbf{AA$\uparrow$}&
    \textbf{Forgetting$\downarrow$}&
    \textbf{FAA$\uparrow$}&
    \textbf{Forgetting$\downarrow$}&
    \textbf{PGD-20$\uparrow$}&
    \textbf{AA$\uparrow$}&
    \textbf{Forgetting$\downarrow$}\\
    \midrule
    \multirow{6}{*}{\textbf{500}}&\textbf{ER+AT}& $11.94_{\pm{0.74}}$& $73.54_{\pm{0.75}}$& $5.66_{\pm{0.31}}$& $5.54_{\pm{0.31}}$& $38.03_{\pm{0.10}}$& $52.71_{\pm{0.96}}$& $28.44_{\pm{1.11}}$& $17.35_{\pm{0.08}}$& $19.56_{\pm
{0.10}}$& $25.67_{\pm{0.26}}$  \\
    ~&\textbf{ER+TRADES}& $7.59_{\pm{0.08}}$& $68.13_{\pm{0.61}}$& $5.43_{\pm{0.05}}$& $5.11_{\pm{0.06}}$& $44.13_{\pm{0.89}}$& $50.75_{\pm{0.42}}$& $20.22_{\pm{0.49}}$& $26.89_{\pm{0.58}}$& $27.69_{\pm{0.56}}$& $20.34_{\pm{0
.72}}$   \\
    ~&\textbf{ER+FAT}& $11.48_{\pm{0.72}}$& $73.99_{\pm{1.18}}$& $5.35_{\pm{0.26}}$& $5.23_{\pm{0.27}}$& $37.26_{\pm{0.62}}$& $56.1_{\pm{1.23}}$& $24.71_{\pm{1.00}}$& $20.01_{\pm{0.85}}$& $22.99_{\pm{0.91}}$& $22.31_{\pm{1.10}}$  \\
    ~&\textbf{ER+LBGAT}& $11.77_{\pm{0.37}}$& $75.1_{\pm{0.40}}$& $6.16_{\pm{0.11}}$& $5.82_{\pm{0.13}}$& $39.77_{\pm{0.18}}$& $42.02_{\pm{2.36}}$& $26.45_{\pm{0.30}}$& $13.99_{\pm{0.83}}$& $14.43_{\pm{0.97}}$& $23.14_{\pm{0.21}}$ \\
    ~&\textbf{ER+Pang~\etal~\cite{pang2022robustness}}& $16.22_{\pm{0.63}}$& $77.71_{\pm{0.44}}$& $0.91_{\pm{0.05}}$& $0.62_{\pm{0.00}}$& $6.13_{\pm{0.16}}$& $68.87_{\pm{0.25}}$& $11.21_{\pm{0.73}}$& $3.23_{\pm{0.42}}$& $7.95_{\pm{0.06}}$& $4.94_{\pm{0.05}}$\\

    \cmidrule(r){2-12}
    ~&\textbf{ER+AT+Ours}& 
    $24.14_{\pm{0.44}}$&$53.03_{\pm{0.3}}$&$7.13_{\pm{0.05}}$&$6.68_{\pm{0.04}}$&$25.81_{\pm{0.13}}$&$56.0_{\pm{0.05}}$&$26.19_{\pm{0.03}}$&$17.95_{\pm{0.04}}$&$20.26_{\pm{0.06}}$&$24.87_{\pm{0.08}}$\\
%      {$17.50_{\pm{0.39}}$}& $66.66_{\pm{0.11}}$& $6.76_{\pm{0.36}}$&  {$6.49_{\pm{0.34}}$}&  {$34.54_{\pm{0.24}}$}& $53.10_{\pm{1.46}}$& $28.59_{\pm{1.51}}$& $17.34_{\pm{0.41}}$& $19.04_{\pm{
% 0.56}}$& $25.77_{\pm{0.66}}$ \\
    ~&\textbf{ER+TRADES+Ours}& 
     {$23.24_{\pm{0.01}}$} & {$24.29_{\pm{0.0}}$} & {$9.93_{\pm{0.37}}$} & {$7.5_{\pm{0.37}}$} & {$11.7_{\pm{3.32}}$} & {$56.68_{\pm{0.44}}$} & {$21.39_{\pm{0.12}}$} & {$27.39_{\pm{0.41}}$} & {$28.5_{\pm{0.34}}$} & {$16.76_{\pm{0.22}}$} \\

    % $14.61_{\pm{1.15}}$&  {$62.63_{\pm{2.25}}$}&  {$7.15_{\pm{0.22}}$}& $6.42_{\pm{0.23}}$& $37.49_{\pm{2.31}}$&  {$54.65_{\pm{0.94}}$}& { $20.56_{\pm{0.51}}$}& {$27.72_{\pm{0.94}}$}&  {$28.50_{\pm{0.55}}$}&  {$18.25_{\pm{1.28}}$}  \\
    \cmidrule(r){1-12}
    \multirow{6}{*}{\textbf{2000}}&\textbf{ER+AT}& $18.77_{\pm{0.18}}$& $65.06_{\pm{0.58}}$& $7.20_{\pm{0.18}}$& $7.01_{\pm{0.18}}$& $33.56_{\pm{0.26}}$& $62.01_{\pm{0.76}}$& $17.97_{\pm{0.80}}$& $21.16_{\pm{0.38}}$& $24.04_{\pm{
0.23}}$& $20.47_{\pm{0.25}}$ \\
    ~&\textbf{ER+TRADES}& $9.50_{\pm{0.24}}$& $70.49_{\pm{0.38}}$& $5.35_{\pm{0.19}}$& $5.01_{\pm{0.17}}$& $42.08_{\pm{0.40}}$& $60.63_{\pm{1.03}}$& $13.78_{\pm{0.90}}$& $26.68_{\pm{0.51}}$& $29.19_{\pm{0.70}}$& $18.60_{\pm{0.54}
}$   \\
    ~&\textbf{ER+FAT}& $17.09_{\pm{1.96}}$& $66.91_{\pm{3.02}}$& $6.12_{\pm{0.40}}$& $5.93_{\pm{0.38}}$& $33.62_{\pm{1.72}}$& $63.88_{\pm{0.02}}$& $15.99_{\pm{0.47}}$& $23.48_{\pm{0.06}}$& $26.75_{\pm{0.05}}$& $17.12_{\pm{0.62}}$  \\
    ~&\textbf{ER+LBGAT}& $20.58_{\pm{0.15}}$& $63.31_{\pm{0.20}}$& $7.93_{\pm{0.17}}$& $7.05_{\pm{0.16}}$& $30.09_{\pm{0.32}}$& $55.77_{\pm{0.23}}$& $25.11_{\pm{0.54}}$& $17.95_{\pm{0.43}}$& $18.88_{\pm{0.54
}}$& $19.18_{\pm{0.48}}$\\
~&\textbf{ER+Pang~\etal~\cite{pang2022robustness}}& $30.10_{\pm{0.53}}$& $61.51_{\pm{1.00}}$& $0.75_{\pm{0.22}}$&$0.51_{\pm{0.02}}$& $4.10_{\pm{0.60}}$& $76.90_{\pm{0.44}}$& $19.60_{\pm{0.32}}$& $4.88_{\pm{0.24}}$&$11.97_{\pm{0.26}}$& $5.25_{\pm{0.20}}$\\
    \cmidrule(r){2-12}
    ~&\textbf{ER+AT+Ours}& 
    $31.93_{\pm{0.07}}$&$40.5_{\pm{0.12}}$&$9.61_{\pm{0.06}}$&$9.16_{\pm{0.04}}$&$17.78_{\pm{0.22}}$&$63.77_{\pm{0.18}}$&$17.16_{\pm{0.31}}$&$23.11_{\pm{0.02}}$&$25.59_{\pm{0.08}}$&$17.57_{\pm{0.07}}$\\
%      {$24.52_{\pm{0.37}}$}&  {$57.28_{\pm{0.34}}$}&  {$8.58_{\pm{0.24}}$}&  {$8.25_{\pm{0.25}}$}&  {$28.44_{\pm{0.18}}$}& $62.42_{\pm{0.28}}$& $18.06_{\pm{0.21}}$& $21.28_{\pm{0.05}}$& $23.88_{\p
% m{0.21}}$& $20.43_{\pm{0.48}}$\\
    ~&\textbf{ER+TRADES+Ours}&
    $28.73_{\pm{1.79}}$&$24.16_{\pm{2.6}}$&$12.75_{\pm{0.34}}$&$11.02_{\pm{0.66}}$&$14.56_{\pm{0.7}}$&$62.01_{\pm{0.89}}$&$13.16_{\pm{1.9}}$&$34.81_{\pm{0.41}}$&$35.36_{\pm{0.95}}$&$11.6_{\pm{0.17}}$\\
    % $19.26_{\pm{0.38}}$& $58.26_{\pm{0.87}}$& $8.26_{\pm{0.14}}$& $7.56_{\pm{0.15}}$& $36.67_{\pm{0.14}}$&  {$63.45_{\pm{0.21}}$}&  {$11.32_{\pm{0.41}}$}&  {$31.66_{\pm{0.21}}$}&  {$33.51_{\pm{0.30}}$}&  {$14.26_{\pm{0.41}}$}  \\
    \bottomrule
    \end{tabular}}
\end{minipage}

\end{table*}

\begin{table*}[]
    \centering % 居中显示
        \caption{Experiments with other data selection-based and logit masking-based continual learning methods. }
    \label{Data_selection_and_logit_masking_std}
    \resizebox{\textwidth}{!}{
    \begin{tabular}{ll ll lll lll}
    \toprule
    \multirow{3}{*}{\textbf{Method}}&\multirow{3}{*}{\textbf{Publication}}
    \multicolumn{4}{c}{\textbf{Class Incremental Setting}} &
    \multicolumn{4}{c}{\textbf{Task Incremental Setting}} \\
    ~&~&\multicolumn{2}{c}{\textbf{Clean Data}}&
    \multicolumn{2}{c}{\textbf{Adversarial Data}}&
    \multicolumn{2}{c}{\textbf{Clean Data}}&
    \multicolumn{2}{c}{\textbf{Adversarial Data}}\\
    ~&~&\textbf{FAA$\uparrow$ }&\textbf{Forgetting$\downarrow$}&
    \textbf{FAA$\uparrow$}&
    \textbf{Forgetting$\downarrow$}&
    \textbf{FAA$\uparrow$}&\textbf{Forgetting$\downarrow$}&
    \textbf{FAA$\uparrow$}&\textbf{Forgetting$\downarrow$}\\
     \midrule
    ER+AT&\multirow{2}{*}{NeurIPS~$2019$}& $28.18_{\pm{0.69}}$ & $80.58_{\pm{1.05}}$ & $17.86_{\pm{0.29}}$ & $69.58_{\pm{1.15}}$ & $84.49_{\pm{0.61}}$ & $10.23_{\pm{0.98}}$ & $44.30_{\pm{1.05}}$ &$36.89_{\pm{1.11}}$\\

    ER+AT+Ours&~& $47.70_{\pm{0.67}}$&$53.19_{\pm{1.87}}$&$18.20_{\pm{0.02}}$&$56.73_{\pm{1.10}}$&$85.40_{\pm{1.28}}$&$9.20_{\pm{1.67}}$&$48.38_{\pm{0.67}}$&$31.68_{\pm{1.49}}$\\
    \midrule
    
    % GSS+AT&  $27.3_{\pm{0.58}}$& $81.25_{\pm{1.11}}$& $16.85_{\pm{0.18}}$& $68.44_{\pm{0.09}}$& $83.93_{\pm{0.52}}$& $10.54_{\pm{1.11}}$& $43.8_{\pm{0.98}}$& $35.63_{\pm{1.46}}$ \\
    GSS+AT&\multirow{2}{*}{NeurIPS~$2019$}&{$27.59_{\pm{0.62}}$} &{$80.78_{\pm{0.99}}$} &{$16.67_{\pm{0.16}}$} &{$68.53_{\pm{0.11}}$} &{$84.41_{\pm{0.10}}$} &{$9.83_{\pm{0.13}}$} &{$44.25_{\pm{0.87}}$} &$34.79_{\pm{0.09}}$\\
    GSS+AT+Ours&~&{$36.93_{\pm{7.13}}$} &{$67.72_{\pm{15.65}}$} &{$16.84_{\pm{0.01}}$} &{$60.04_{\pm{16.20}}$} &{$85.57_{\pm{0.56}}$} &{$8.86_{\pm{1.84}}$} &{$47.11_{\pm{0.04}}$} &$31.83_{\pm{0.36}}$\\
    \midrule
    ASER+AT&\multirow{2}{*}{AAAI~$2021$}&{$18.85_{\pm{0.00}}$} &{$87.78_{\pm{0.34}}$} &{$14.06_{\pm{0.57}}$} &{$65.57_{\pm{0.01}}$} &{$73.87_{\pm{6.23}}$} &{$19.01_{\pm{13.46}}$} &{$30.65_{\pm{14.44}}$} &$44.85_{\pm{30.80}}$\\
    ASER+AT+Ours&~&{$24.45_{\pm{0.03}}$} &{$81.73_{\pm{0.60}}$} &{$14.91_{\pm{0.07}}$} &{$62.74_{\pm{0.66}}$} &{$77.70_{\pm{0.08}}$} &{$15.21_{\pm{0.43}}$} &{$34.50_{\pm{0.15}}$} &$38.55_{\pm{0.39}}$\\
    \midrule
    X-DER+AT&\multirow{2}{*}{TPAMI~$2022$}&{$34.04_{\pm{0.81}}$} &{$25.13_{\pm{16.25}}$} &{$16.82_{\pm{0.95}}$} &{$27.84_{\pm{17.33}}$} &{$80.80_{\pm{0.44}}$} &{$4.96_{\pm{2.74}}$} &{$60.83_{\pm{0.31}}$} &$10.99_{\pm{0.65}}$\\
    X-DER+AT+Ours&~&{$43.25_{\pm{0.09}}$} &{$20.77_{\pm{2.56}}$} &{$17.22_{\pm{0.00}}$} &{$18.56_{\pm{11.86}}$} &{$84.87_{\pm{0.00}}$} &{$1.74_{\pm{0.02}}$} &{$61.68_{\pm{0.00}}$} &$7.03_{\pm{1.50}}$\\
    
    % ASER+AT&  $14.3_{\pm{1.37}}$& $66.26_{\pm{17.44}}$& $6.14_{\pm{0.78}}$& $40.15_{\pm{62.91}}$& $60.06_{\pm{21.55}}$& $10.3_{\pm{0.65}}$& $17.18_{\pm{11.69}}$& $27.35_{\pm{44.24}}$\\

    % ER-ACE+AT  & $52.11_{\pm{1.31}}$ & $29.35_{\pm{4.13}}$ & $13.99_{\pm{0.30}}$ & $25.92_{\pm{2.97}}$ & $87.37_{\pm{0.24}}$ & $7.76_{\pm{0.08}}$ & $44.65_{\pm{0.81}}$ &$26.74_{\pm{2.34}}$\\

    % XDER+AT  & $45.73_{\pm{4.3}}$& $20.97_{\pm{1.34}}$& $12.28_{\pm{0.81}}$& $18.09_{\pm{2.45}}$& $86.89_{\pm{0.69}}$& $8.08_{\pm{0.53}}$& $46.17_{\pm{3.4}}$& $21.12_{\pm{1.43}}$\\

\bottomrule
\end{tabular}}
\end{table*}
\begin{table*}[]
    \centering % 居中显示
     \caption{Experiment results on S-Tiny-ImageNet dataset and model architecture is ResNet18.
    Following~\cite{buzzega2020dark}, we choose two buffer sizes of 200 and 5120.
    Here PGD-20 and AA are adversarial data Final Average Accuracy (FAA) generated by PGD-20 and Auto Attack (AA) respectively. Forgetting of adversarial data is computed based on PGD-20. \textbf{Bold} represents the best experimental results for the same settings. With the addition of ours, model performance can be improved across the board.}
    \label{Main-TinyImg_std}
    \resizebox{\textwidth}{!}{

    \begin{tabular}{llllllllllll}
    \toprule
    \multirow{3}{*}{\textbf{Buffer Size}} &
    \multirow{3}{*}{\textbf{Methods}} &
    \multicolumn{5}{c}{\textbf{Class Incremental Setting}} &
    \multicolumn{5}{c}{\textbf{Task Incremental Setting}} \\
    ~&~&\multicolumn{2}{c}{\textbf{Clean Data}}&
    \multicolumn{3}{c}{\textbf{Adversarial Data}}&
    \multicolumn{2}{c}{\textbf{Clean Data}}&
    \multicolumn{3}{c}{\textbf{Adversarial Data}}\\
    ~&~&\textbf{FAA$\uparrow$ }&\textbf{Forgetting$\downarrow$}&
    \textbf{PGD-20$\uparrow$}&
    \textbf{AA$\uparrow$}&
    \textbf{Forgetting$\downarrow$}&
    \textbf{FAA$\uparrow$}&
    \textbf{Forgetting$\downarrow$}&
    \textbf{PGD-20$\uparrow$}&
    \textbf{AA$\uparrow$}&
    \textbf{Forgetting$\downarrow$}\\
    \midrule
    \multirow{2}{*}{\textbf{200}}&\textbf{ER+TRADES} & $5.50_{\pm{0.41}}$ & $54.67_{\pm{0.13}}$ & $2.04_{\pm{0.35}}$ & $1.92_{\pm{0.35}}$ & $22.62_{\pm{0.21}}$ & $23.51_{\pm{1.38}}$ & $34.72_{\pm{1.15}}$ & $5.28_{\pm{0.73}}$ & $6.48_{\pm{0.91}}$ & $19.10_{\pm{0.42}}$    \\
    ~&\textbf{ER+TRADES+Ours}&\pmb{$7.35_{\pm{0.43}}$} &\pmb{$52.38_{\pm{0.22}}$} &\pmb{$2.22_{\pm{0.08}}$} &\pmb{$2.05_{\pm{0.03}}$} &\pmb{$20.79_{\pm{0.14}}$} &\pmb{$25.58_{\pm{0.73}}$} &\pmb{$34.94_{\pm{1.44}}$} &\pmb{$6.24_{\pm{0.30}}$} &\pmb{$7.60_{\pm{0.26}}$} &\pmb{$18.41_{\pm{0.20}}$}  \\
    \cmidrule(r){1-12}
    \multirow{2}{*}{\textbf{5120}}&\textbf{ER+TRADES}& $7.24_{\pm{0.39}}$ & $55.69_{\pm{1.06}}$ & $2.39_{\pm{0.16}}$ & $2.21_{\pm{0.14}}$ & $21.59_{\pm{0.91}}$ & $41.36_{\pm{1.07}}$ & $18.16_{\pm{1.74}}$ & $11.01_{\pm{0.92}}$ & $13.71_{\pm{0.78}}$ & $12.61_{\pm{1.45}}$ \\
    ~&\textbf{ER+TRADES+Ours}&\pmb{$10.95_{\pm{0.8}}$} &\pmb{$51.63_{\pm{1.11}}$} &\pmb{$3.01_{\pm{0.24}}$} &\pmb{$2.79_{\pm{0.25}}$} &\pmb{$21.74_{\pm{0.6}}$} &\pmb{$44.81_{\pm{0.13}}$} &\pmb{$15.20_{\pm{0.08}}$} &\pmb{$12.92_{\pm{0.16}}$} &\pmb{$16.21_{\pm{0.06}}$} &\pmb{$12.33_{\pm{0.42}}$}\\
    \bottomrule
    % \midrule
    \end{tabular}
    }
\end{table*}
\begin{table*}[]
 \caption{Adaptive Attack for ER+TRADES+ours. All the attack methods in the table incorporate the same logit calibration as in the training phase of our model. Forgetting is based on PGD-20. Results show our method still maintains decent robustness.}
    \label{adaptive_std}
    \centering % 居中显示
    \scalebox{1.15}{
    \begin{tabular}{ll lll lll}
    \toprule
    \multirow{2}{*}{\textbf{Dataset}} &
    \multirow{1}{*}{\textbf{Buffer}}&
    \multicolumn{3}{c}{\textbf{Class Incremental Setting}} &
    \multicolumn{3}{c}{\textbf{Task Incremental Setting}} \\
    ~&\multirow{1}{*}{\textbf{Size}}&\textbf{ PGD-20 }&
    \textbf{ AA}&
    \textbf{Forgetting}&
    \textbf{ PGD-20 }&
    \textbf{AA}&
    \textbf{Forgetting}\\
    \midrule
    \multirow{2}{*}{\textbf{CIFAR-10}}&\textbf{200}&
    $23.99_{\pm{1.36}}$&$41.76_{\pm{0.00}}$&$26.43_{\pm{8.04}}$&$58.18_{\pm{0.17}}$&$58.32_{\pm{0.26}}$&$15.40_{\pm{0.26}}$\\
    % $23.13_{\pm{1.87}}$ & $41.39_{\pm{4.58}}$ & $38.35_{\pm{8.56}}$& $59.41_{\pm{0.63}}$ &$59.60_{\pm{0.63}}$& $14.16_{\pm{1.28}}$ \\
    ~&\textbf{5120}&
    $27.50_{\pm{2.80}}$&$35.29_{\pm{0.52}}$&$1.53_{\pm{0.69}}$&$65.59_{\pm{3.26}}$&$60.69_{\pm{0.50}}$&$5.89_{\pm{3.20}}$\\
    % $23.62_{\pm{6.77}}$ & $37.22_{\pm{12.19}}$ & $41.96_{\pm{12.00}}$ & $69.27_{\pm{2.23}}$ & $69.35_{\pm{2.24}}$& $5.31_{\pm{0.75}}$\\
    \midrule
    \multirow{2}{*}{\textbf{CIFAR-100}}&\textbf{500}&
    $9.91_{\pm{0.52}}$&$20.61_{\pm{0.98}}$&$13.10_{\pm{1.52}}$&$26.84_{\pm{0.94}}$&$28.20_{\pm{0.72}}$&$17.13_{\pm{0.79}}$\\
    % $7.40_{\pm{0.54}}$ & $11.83_{\pm{1.22}}$ & $38.78_{\pm{1.37}}$ & $27.64_{\pm{0.96}}$ & $28.84_{\pm{0.56}}$ & $18.13_{\pm{1.28}}$\\
    ~&\textbf{2000}&
    $13.68_{\pm{0.93}}$&$25.85_{\pm{0.73}}$&$15.33_{\pm{1.02}}$&$34.83_{\pm{0.62}}$&$35.72_{\pm{0.84}}$&$11.59_{\pm{0.42}}$\\
    % $8.68_{\pm{0.20}}$ & $16.15_{\pm{0.38}}$ & $37.87_{\pm{0.08}}$ & $31.48_{\pm{0.18}}$ & $33.83_{\pm{0.28}}$& $14.21_{\pm{0.34}}$\\
\bottomrule
\end{tabular}}
   
\end{table*}

% \begin{table*}[]
%     \caption{Adaptive Attack for ours}
%     \label{adaptive}
%     \centering % 居中显示
%     \scalebox{0.7}{
%     \begin{tabular}{lllllllllll}
%     \toprule
%     \multirow{2}{*}{\textbf{Dataset}} &
%     \multirow{2}{*}{\textbf{Buffer Size}}&
%     \multirow{2}{*}{\textbf{Baseline}} &
%     \multicolumn{4}{c}{\textbf{Class Incremental Setting}} &
%     \multicolumn{4}{c}{\textbf{Task Incremental Setting}} \\
%     ~&~&~&\textbf{ PGD-20 }&
%     \textbf{ AA}&
%     \textbf{ PGD-20 Forgetting}&
%     \textbf{ AA Forgetting}&
%     \textbf{ PGD-20 }&
%     \textbf{AA}&
%     \textbf{PGD-20 Forgetting}&
%     \textbf{AA Forgetting}\\
%     \midrule
%     \multirow{4}{*}{\textbf{CIFAR-10}}&\multirow{2}{*}{\textbf{200}}&
%     \textbf{AT}&0 & 0 & 0 & 0& 0 & 0& 0 & 0 \\
%     ~&~&\textbf{TRADES}&$23.13_{\pm{1.87}}$ & 0 & $38.35_{\pm{8.56}}$ & 0 & $59.41_{\pm{0.63}}$ & 0& $14.16_{\pm{1.28}}$ & 0\\
%     ~&\multirow{2}{*}{\textbf{5120}}&
%     \textbf{AT}&0 & 0 & 0 & 0& 0 & 0& 0 & 0 \\
%     ~&~&\textbf{TRADES}&$23.62_{\pm{6.77}}$ & 0 & $41.96_{\pm{12.00}}$ & 0 & $69.27_{\pm{2.23}}$ & 0& $5.31_{\pm{0.75}}$& 0\\
%     \midrule
%     \multirow{4}{*}{\textbf{CIFAR-100}}&\multirow{2}{*}{\textbf{500}}&
%     \textbf{AT}&0 & 0 & 0 & 0& 0 & 0& 0 & 0 \\
%     ~&~&\textbf{TRADES}&0 & 0 & 0 & 0 & 0 & 0& 0 & 0\\
%     ~&\multirow{2}{*}{\textbf{2000}}&
%     \textbf{AT}&0 & 0 & 0 & 0& 0 & 0& 0 & 0 \\
%     ~&~&\textbf{TRADES}&0 & 0 & 0 & 0 & 0 & 0& 0 & 0\\
% \bottomrule
% \end{tabular}}
% \end{table*}
\noindent \textbf{Results with Standard Error.}
In this section, we provide results with mean and standard error.
In the task incremental setting, we observe more stable experimental results compared to the class incremental setting. Furthermore, our approach achieves consistent improvements in the majority of cases.

\noindent \textbf{Accuracy during Training in Split-CIFAR10.}
Figure~\ref{fig:task_acc_cifar10} shows FAAs of different continual training phrases of ER+AT, ER+TRADES, and their combination with us.
In the vast majority of experiments, our proposed method can improve the performance of the baseline models at each incremental training stage.
Despite a minor decline in FAA on clean samples compared to baselines under the task incremental setting with a buffer size of $5,120$, this is due to the balance between robustness and performance and the forgetting alleviation from AFLC diminishes as buffer size increases.
For FAA, this is attributed to that the RAER component designed for robustness improvement can adversely affect clean data performance, exacerbated by the large buffer size.
The trade-off between standard and robust accuracy is an expected consequence of adversarial training, wherein improved adversarial robustness typically incurs some cost to natural sample performance.
Nonetheless, our approach still confers substantial gains in adversarial robustness with limited sacrifice of conventional accuracy compared to baselines, as elucidated by the buffer size analysis on the interaction between RAER and AFLC.
In addition, AFLC aims to mitigate the phenomenon of forgetting which hinders the learning of current tasks. Therefore, in the initial task, there might be a slight performance decline due to AFLC. However, the benefits of AFLC become prominent in later stages, leading to improved robustness.

\begin{figure*}[t]
  \centering
  \includegraphics[width=1.0\linewidth]{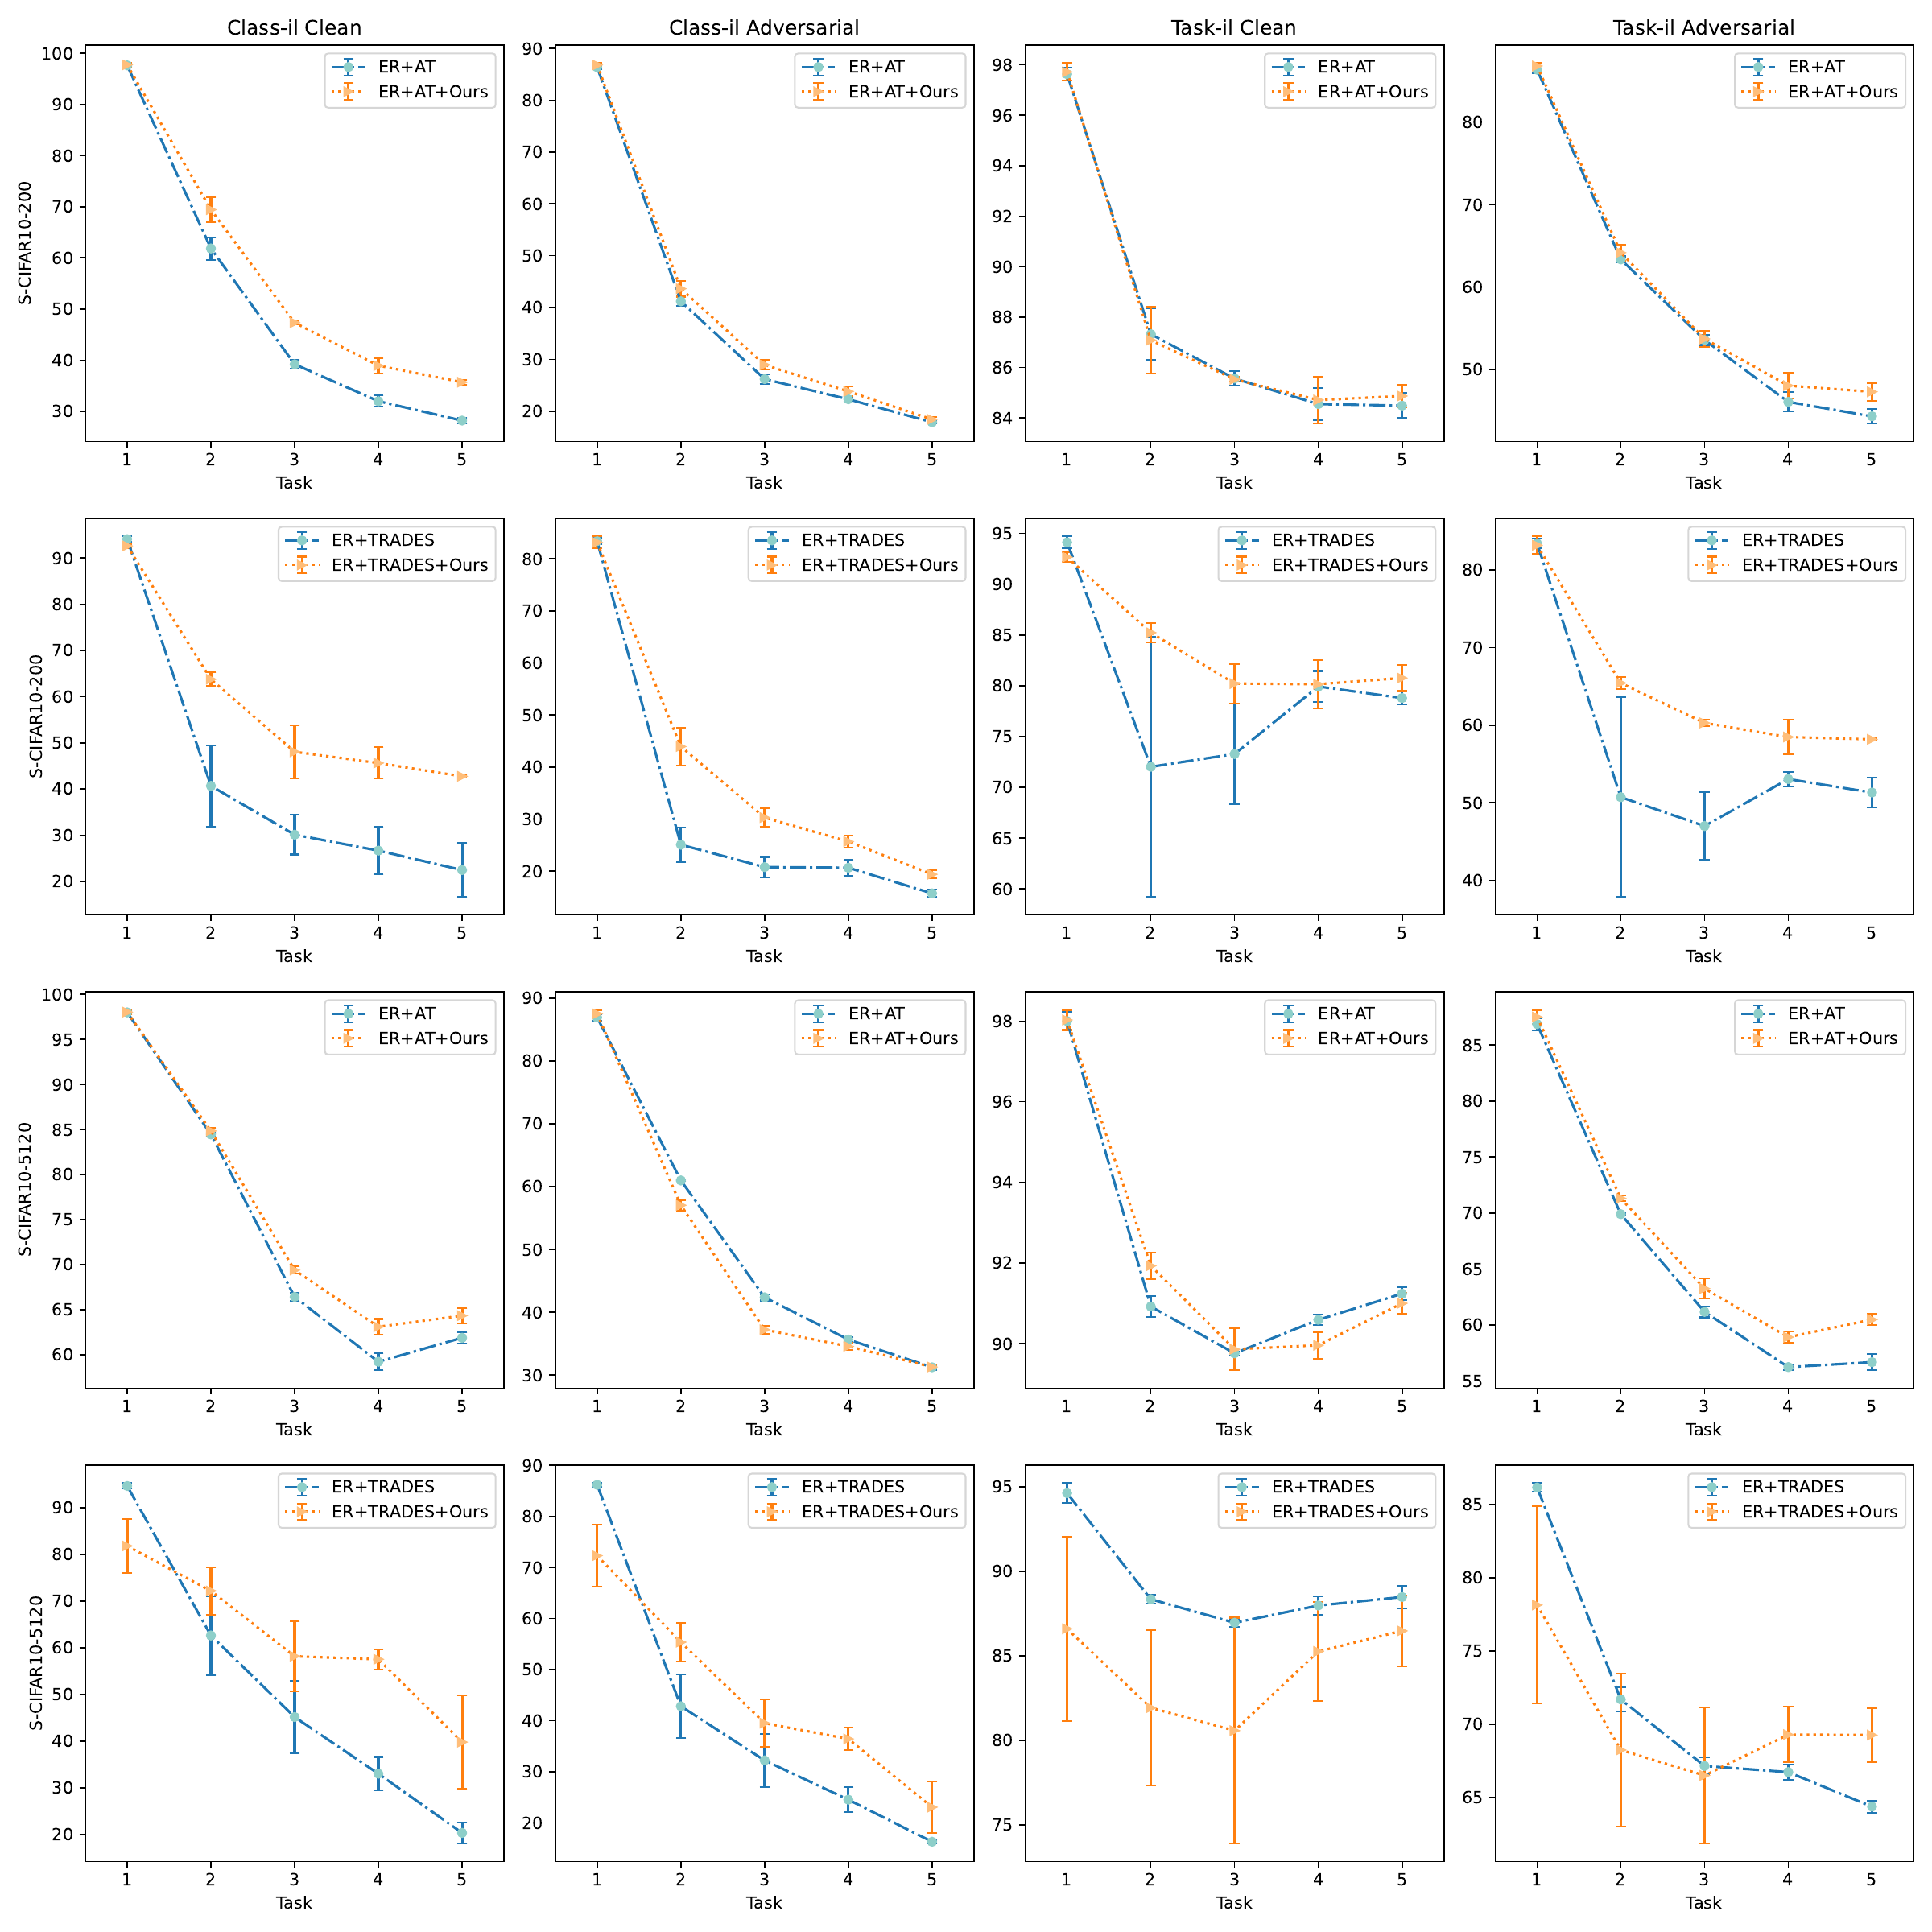}
  \caption{Accuracy curves on the Split-CIFAR10 with buffer size $200$, and $5,120$ settings.
  The plots' x-axis denotes the total number of tasks trained cumulatively up to each learning stage. The y-axis shows the average accuracy of the current task at each respective stage.
  The results demonstrate consistent improvements across most stages of continual learning when our proposed approach is combined with the baseline model.
  }
  \label{fig:task_acc_cifar10}
\end{figure*}
\clearpage
